# Supplementary material for: Estimating efficacy of measles supplementary immunization activities via discrete-time modeling of disease incidence time series
Source: arXiv:2010.08875 ancillary file (2020-10-17)
Supplement: Supplementary file 1 [file SuppInfo.pdf]

# Supporting Information for "Estimating efficacy of measles supplementary immunization activities via discrete-time modeling of disease incidence time series"

Tracy Qi Dong[1] and Jon Wakefield[1,2]

[1] Department of Biostatistics, University of Washington
[2] Department of Statistics, University of Washington

## Web Appendix A

### The susceptible-infected-recovered (SIR) model

Historically, infectious disease data were analyzed using deterministic models based on differential equations (Anderson et al., 1992). Models are set up based on a set of compartments in which individuals undergo homogeneous mixing.

A widely used compartmental model is the susceptible-infected-recovered (SIR) model, depicted below.

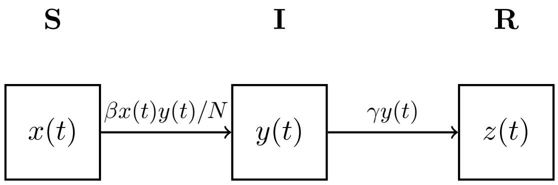


This approach is typically used when the number of disease counts is large, and the integer numbers in the constituent $S$, $I$ and $R$ compartments are taken to be continuous. Let $x(t)$, $y(t)$, $z(t)$ be the number of *susceptibles*, *infected*, *recovered* individuals at time $t$ in a *closed population* of size $N$. The *hazard rate (force of infection)* is

$$\underbrace{\lambda^{\dagger}(t)}_{\text{Hazard}} = \underbrace{c(N)}_{\text{Contact Rate}} \times \underbrace{\frac{y(t)}{N}}_{\text{Prevalence}} \times \underbrace{p_I}_{\text{Infection Prob}} .$$

Two common forms for the contact rate (Begon et al., 2002) are

$$c(N) = \begin{cases} c_{\text{FD}} & \text{Frequency Dependent,} \\ Nc_{\text{DD}} & \text{Density Dependent.} \end{cases}$$

The *frequency-dependent* model is often used, particularly for childhood infections when the most relevant contact group is the classroom, whose size will be of the same order, regardless of the population size. Under *frequency dependency*,

$$\lambda^{\dagger}(t) = \beta y(t)/N,$$

where $\beta = c_{\text{FD}} \times p_{\text{I}}$.

The deterministic SIR model is defined through classic *mass-action* (Anderson et al., 1992). With *frequency dependent* transmission, we have the following set of ordinary differential equations:

$$\begin{aligned}
\frac{dx(t)}{dt} &= -\frac{\beta x(t)y(t)}{N}, \\
\frac{dy(t)}{dt} &= \frac{\beta x(t)y(t)}{N} - \gamma y(t), \\
\frac{dz(t)}{dt} &= \gamma y(t),
\end{aligned}$$

with *infection rate* $\beta$ and *recovery rate* $\gamma$.

The discrete-time stochastic SIR model treats the current disease counts as a function of previous counts on a regular time scale. One may choose the time scale to be the transmission dynamics time (i.e., latency plus infectious periods) or the generation time (i.e., time from infection of a primary case to infection of a secondary case infected by the primary case). For example, often, but not always, 2 weeks is used for measles.

## The time-series SIR (TSIR) framework

The time-series SIR (TSIR) model is a discrete-time stochastic SIR model first described in Finkenstädt and Grenfell (2000). It was extended in a series of subsequent papers (Bjørnstad et al., 2002; Grenfell et al., 2002; Glass et al., 2003; Morton and Finkenstädt, 2005) and has been used to understand measles and rubella transmission in a variety of settings (Ferrari et al., 2008; Metcalf et al., 2011; Mahmud et al., 2017; Metcalf et al., 2013). Under this framework, the infected individuals are assumed to be infectious for one time unit before becoming removed. Therefore, we lose the recovery rate parameter and incidence is assumed equal to prevalence.

A simple model for the susceptibles at time $t$, denoted $X_t$, in the context of measles without vaccination is

$$X_t = X_{t-1} - Y_t + B_{t-d}$$

where $Y_t$ is the number of infected individuals, and $B_{t-d}$ is the number of births $d$ time units previously, with $d$ chosen to be the number of time units for which maternally derived immunity lasts.

The TSIR framework usually uses a negative binomial model for the number of infected individuals. It arises as the distribution of the population size in a linear birth process (Feller, 1950; Cox and Miller, 1977). Details of this derivation can be found in Wakefield et al. (2019). A classic form of the model for the number of infected individuals $Y_t$ is

$$Y_t | Y_{t-1} = y_{t-1}, X_{t-1} = x_{t-1} \sim \text{NegBin}\left(\mu_t, y_{t-1}\right)$$

with

$$\mu_t = \frac{\beta y_{t-1}^{\alpha} x_{t-1}}{N},$$

where $\beta$ is the infection rate parameter. The power parameter $\alpha$ is included to allow for deviations from mass action and to account for the discrete-time approximation to the continuous time model (Glass et al., 2003).

# Web Appendix B

We present a simulation study to further investigate the behavior of the reporting rate estimates from the OLS procedure outlined in Section 2.2.1 of the main paper. We first simulate one set of semi-monthly time series for total population ($N$) and adjusted births ($Bstar$), each of length 15 years (i.e., 360 semi-months), shown below.

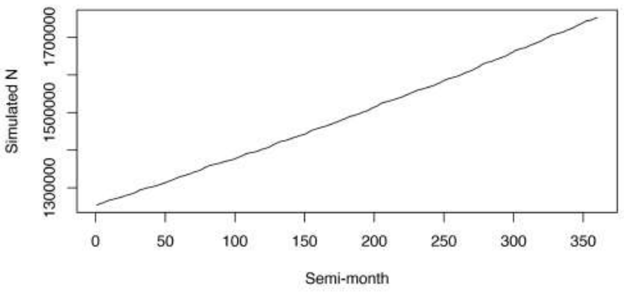


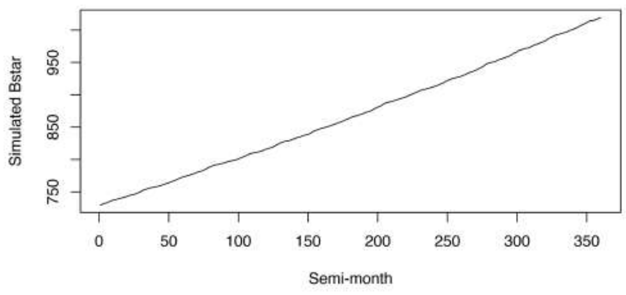


Next, we simulate 100 sets of semi-monthly time series for the susceptible population ($S$) and the underlying true incidence ($I$) using the same parameter values described in Section 3 of the main paper, each with a different starting value. The resultant simulated data are shown below, with each line representing one simulated time series.

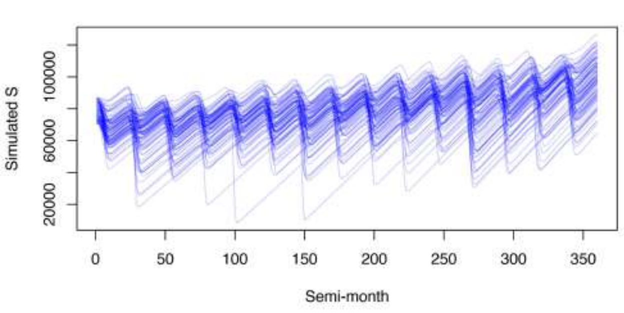


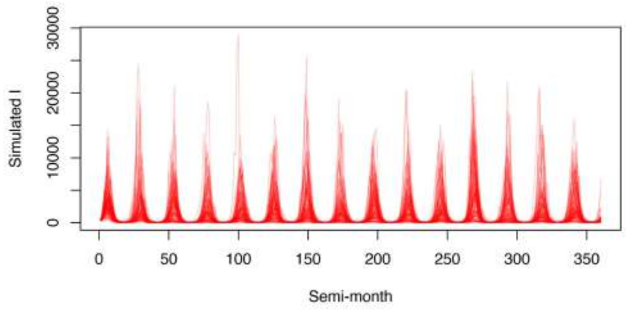


Finally, for each simulated semi-monthly time series of true incidence $I$, we simulate a monthly time series of (observed) reported incidence ($Cstar$) from using binomial distribution with reporting probability $\rho = 0.5$. The results are shown below.

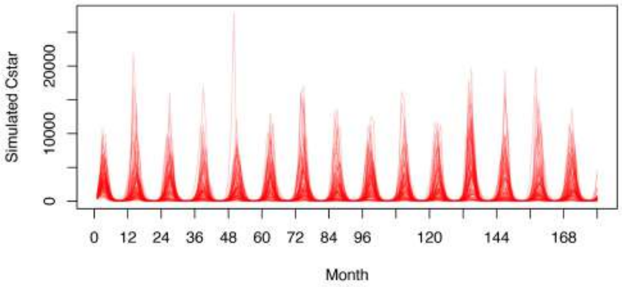


To investigate how reporting rate estimation changes with the lengths and shapes of the time series used to fit the OLS regression, we consider the following sets of *start months* and *lengths* (in months):

- *Start month*: 2, 4, 6, 8, 10, 12
- *Length* (in months): 10, 30, 50, 70, 90, 110, 130, 150

For each combination of *start month* and *length*, and for each simulated reported incidence and adjusted births time series, we subset the data that starts from the *start month* and ends after the number of months specified by *length*, and implement the OLS procedure to obtain an estimate of the reporting rate $\hat{\rho}$. As such, for each combination of *start month* and *length*, we have 100 estimates. We calculate the bias to be the mean of the deviations of $\hat{\rho}$ from the true $\rho = 0.5$, and plot the bias for each scenario. The results are shown below.

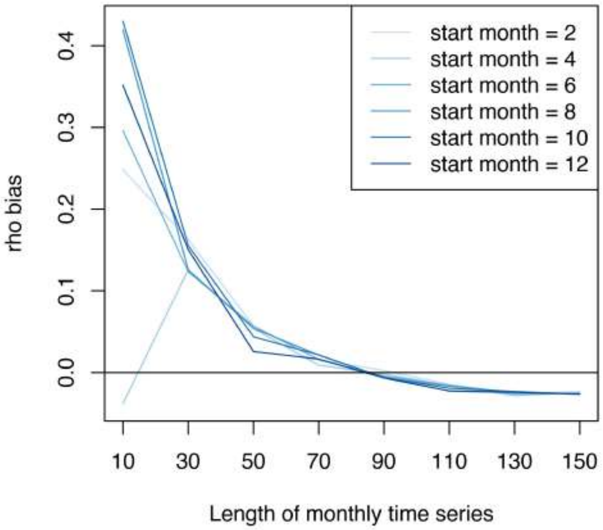

We see that when the lengths of the time series data used to fit OLS regression are short, the procedure generally over-estimates the reporting rate. This is likely a result of the small sample size of the data. As *length* increases, the magnitude of over-estimation generally decreases, until when *length* is between 70 and 90, the bias reaches 0. After that, as *length* increases, the procedure produces under-estimated results and the magnitude of under-estimation eventually approaches a constant value. This pattern generally holds for each *start month* value except for one (when *length* = 4). We repeated the simulation study with several additional reporting rate parameter values ($\rho = 0.01$, 0.1, 0.3 and 0.7), the results show similar patterns.

The reason why the OLS procedure would under-estimate the reporting rate parameter $\rho = \frac{1}{\kappa}$ even when there is enough data for fitting the regression model, is that the cumulative reported incidence and the susceptible population dynamics are correlated. Recall that the relationship that motivates the OLS regression for estimating $\rho = \frac{1}{\kappa}$ is the Equation (12) in the main paper:

$$Y_m = \beta_0 + \kappa X_m + U_m$$

where $Y_m = \sum_{i=1}^{m} B_i$ are the cumulative adjusted births, $X_m = \sum_{i=1}^{m} C_i$ are the cumulative reported incidence, $\beta_0 = \bar{S} - S_0$ is the difference between $S_0$ and $\bar{S}$, and $U_m = S_m - \bar{S}$ are the deviations of $S_m$ from the average $\bar{S}$.

When fitting an OLS regression with the cumulative adjusted birth $Y_m$ as the response variable and the cumulative reported incidence $X_m$ as the explanatory variable, the slope parameter, denoted $\kappa^*$, can be expressed as the ratio of the covariance between $X_m$ and $Y_m$ and the variance of $X_m$:

$$\kappa^* = \frac{Cov(X_m, Y_m)}{Var(X_m)}$$

Replacing $Y_m$ with Equation (12) of the main paper, we have

$$\begin{aligned}
\kappa^* &= \frac{Cov(X_m, \beta_0 + \kappa X_m + U_m)}{Var(X_m)} \\
&= \frac{\kappa Var(X_m) + Cov(X_m, U_m)}{Var(X_m)} \\
&= \kappa + \frac{Cov(X_m, U_m)}{Var(X_m)}
\end{aligned}$$

If $X_m$ and $U_m$ are not correlated, then $Cov(X_m, U_m) = 0$ and the OLS regression should produce unbiased estimate for $\kappa$. However, in our case, $X_m$ and $U_m$ are positively correlated, as shown in the figure below: for each scenario, we plot the average of the empirical correlation between the cumulative reported incidence $X_m$ and the deviance of susceptible time series from its mean $U_m$. We see that the average empirical correlation is positive under all scenarios

except for two where the time series are very short. Therefore, when the time series is long and sample size is large, the covariance between $X_m$ nad $U_m$ is generally positive, i.e., $Cov(X_m, U_m) > 0$. As a result, the OLS regression would over-estimate $\kappa$ and hence, under-estimate the reporting rate $\rho = \frac{1}{\kappa}$.

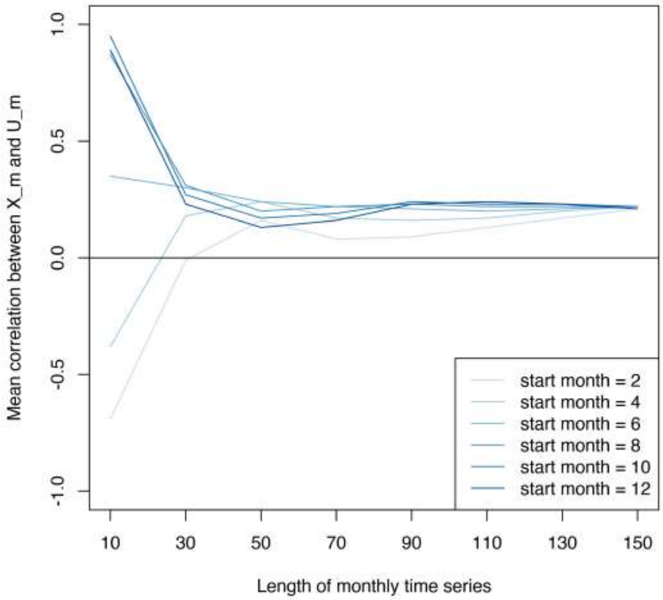

# Web Figure 1

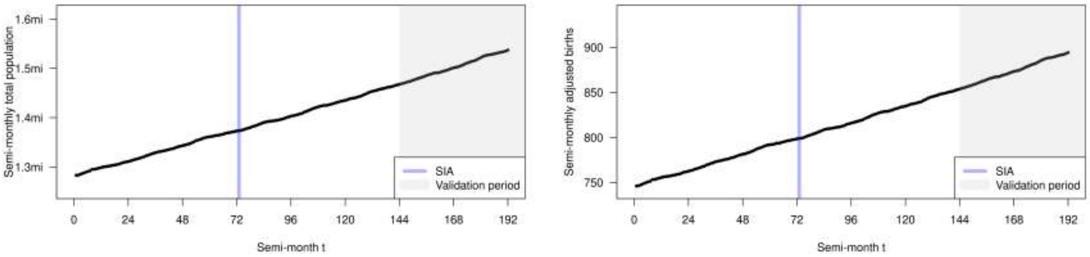


Web Figure 1: The simulated semi-monthly time series of total population (left) and adjusted births entering the susceptible population (right).

# Web Figure 2

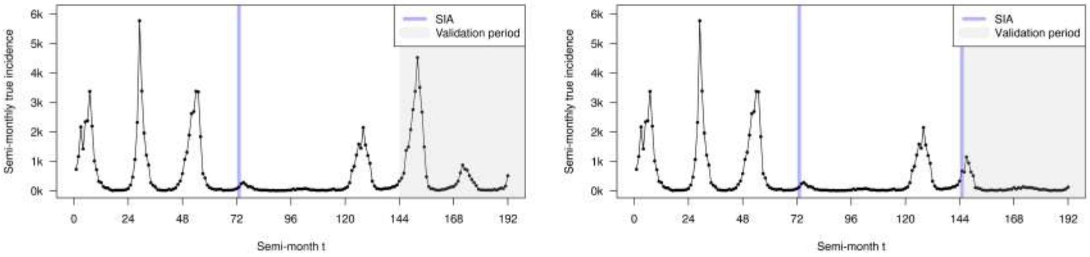


Web Figure 2: The simulated semi-monthly time series of underlying incidence, without (left) and with (right) a "planned" SIA at the beginning of the forecast period.

# Web Figure 3

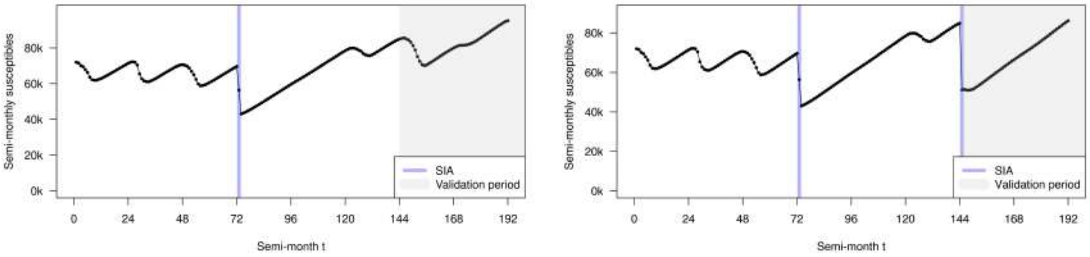


Web Figure 3: The simulated semi-monthly time series of underlying susceptible population, without (left) and with (right) a "planned" SIA at the beginning of the forecast period.

# Web Figure 4

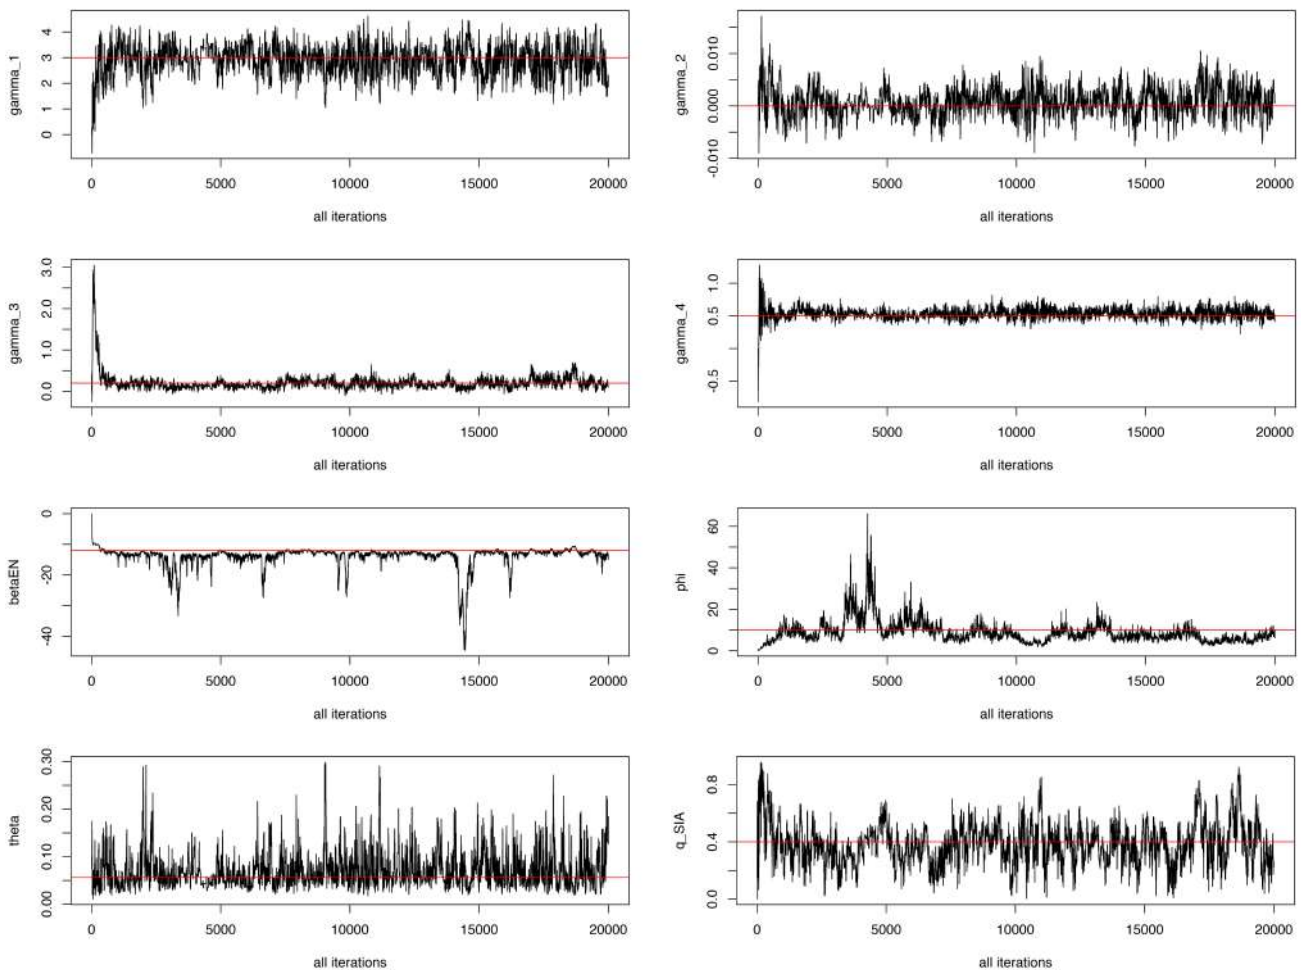


Web Figure 4: Traceplots of posterior samples of model parameters in the simulation study computed with uncertainty propagation for when the reporting rate $\rho = 0.01$.

## Web Figure 5

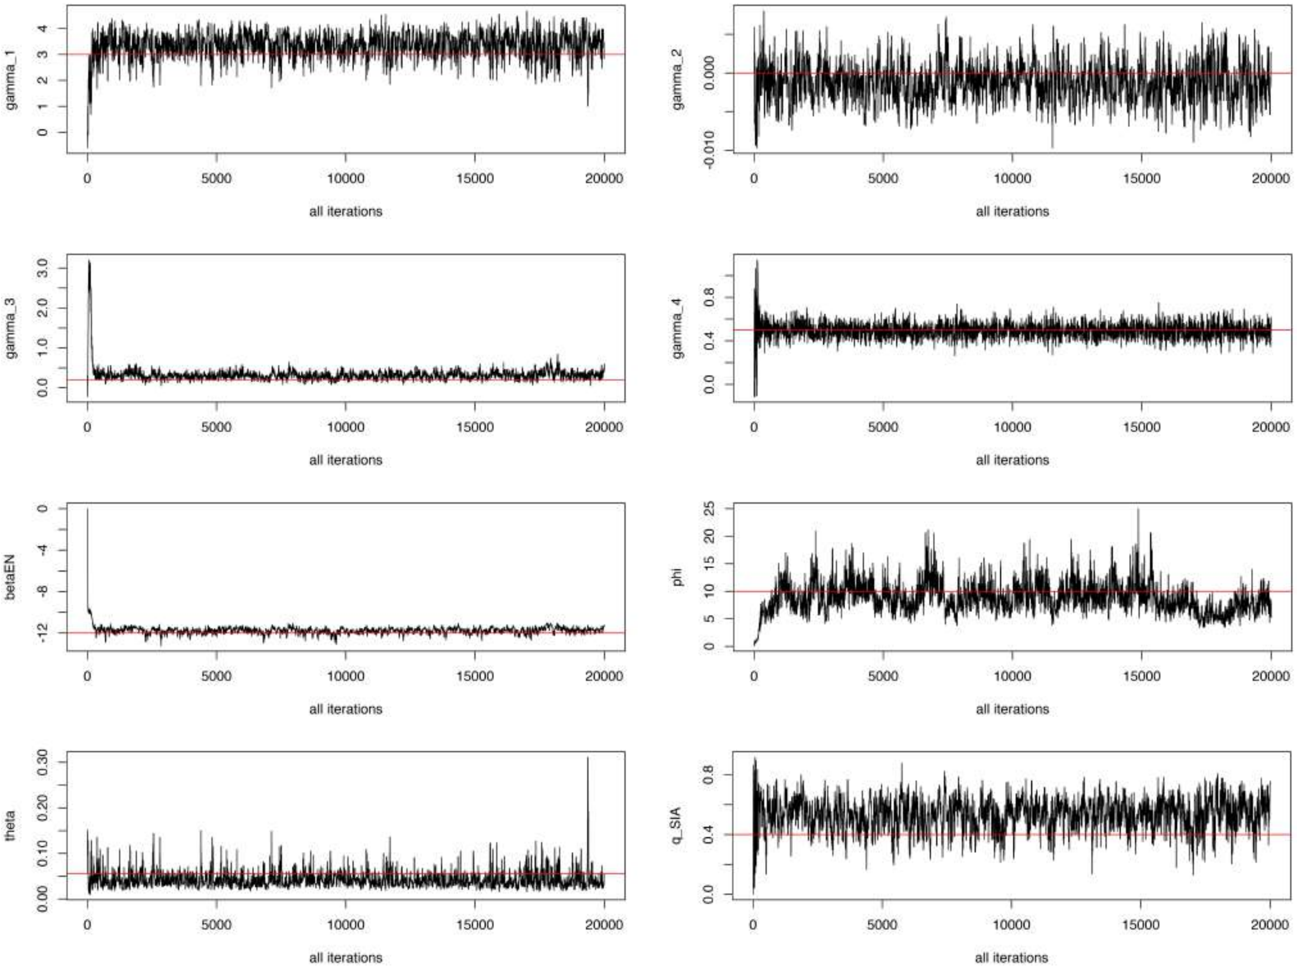


Web Figure 5: Traceplots of posterior samples of model parameters in the simulation study computed with uncertainty propagation for when the reporting rate $\rho = 0.1$.

# Web Figure 6

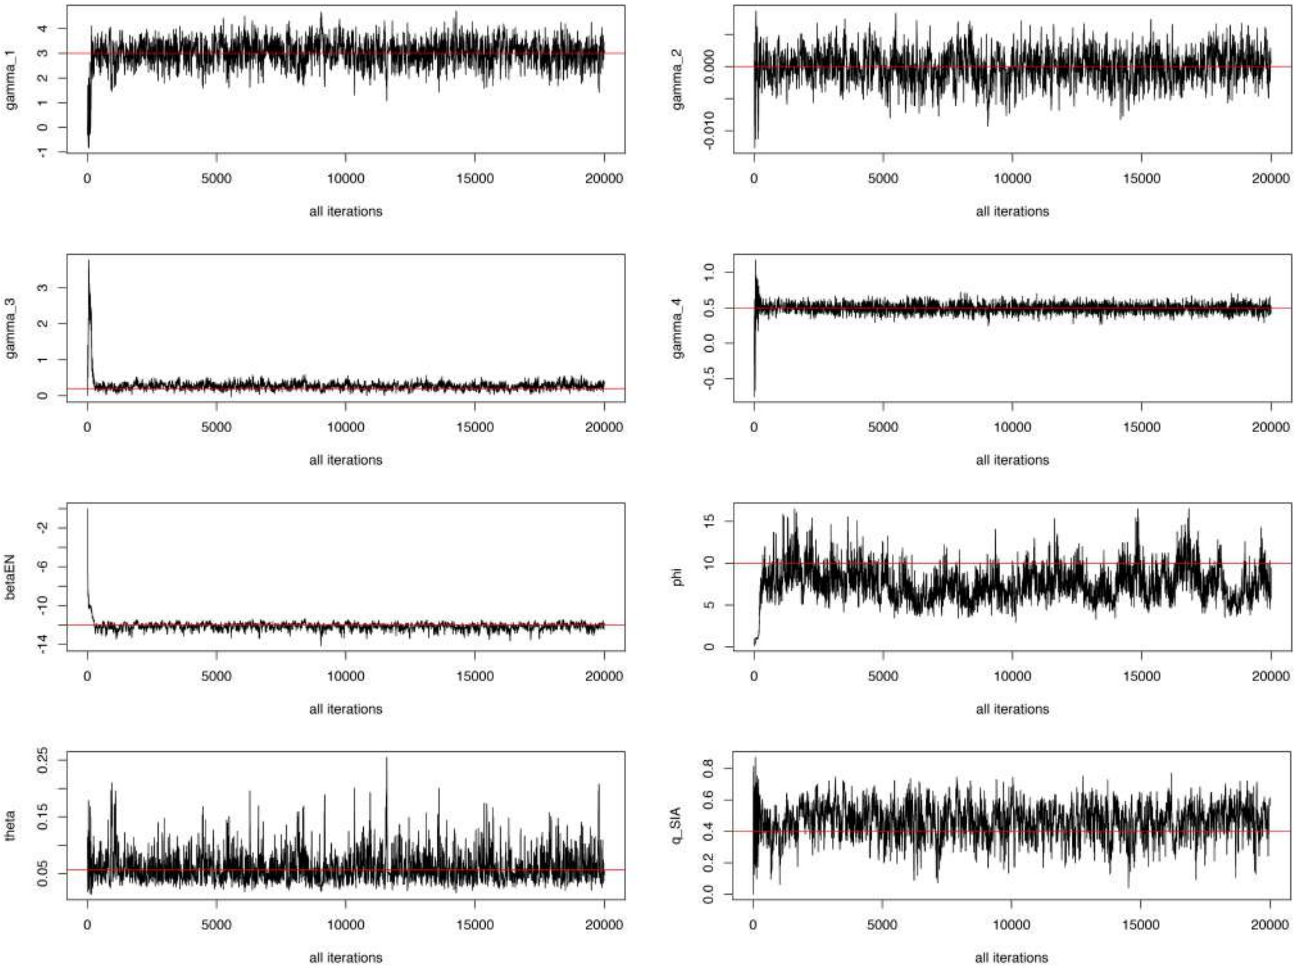


Web Figure 6: Traceplots of posterior samples of model parameters in the simulation study computed with uncertainty propagation for when the reporting rate $\rho = 0.3$.

## Web Figure 7

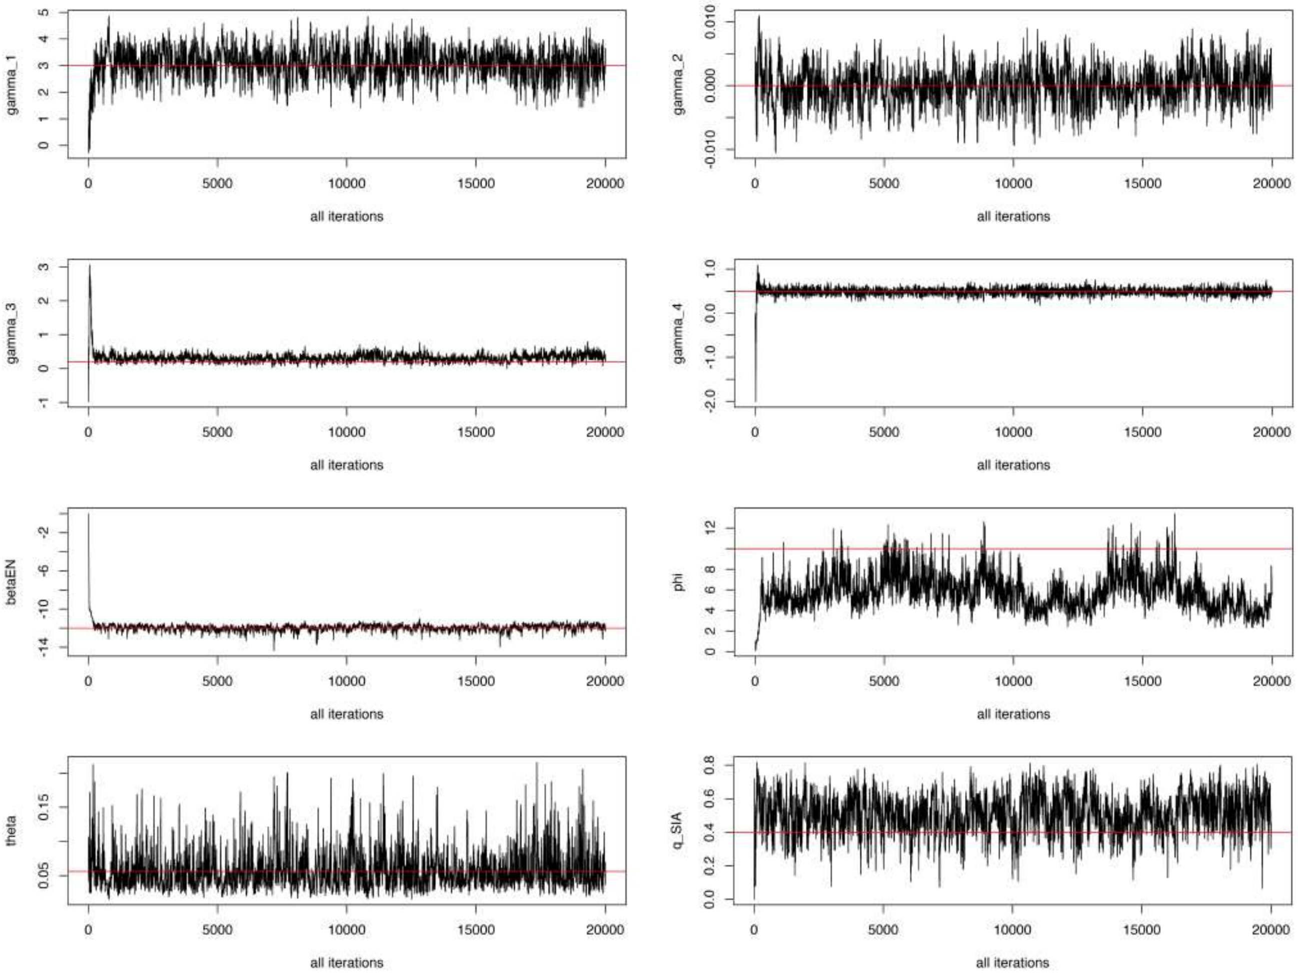


Web Figure 7: Traceplots of posterior samples of model parameters in the simulation study computed with uncertainty propagation for when the reporting rate $\rho = 0.5$.

## Web Figure 8

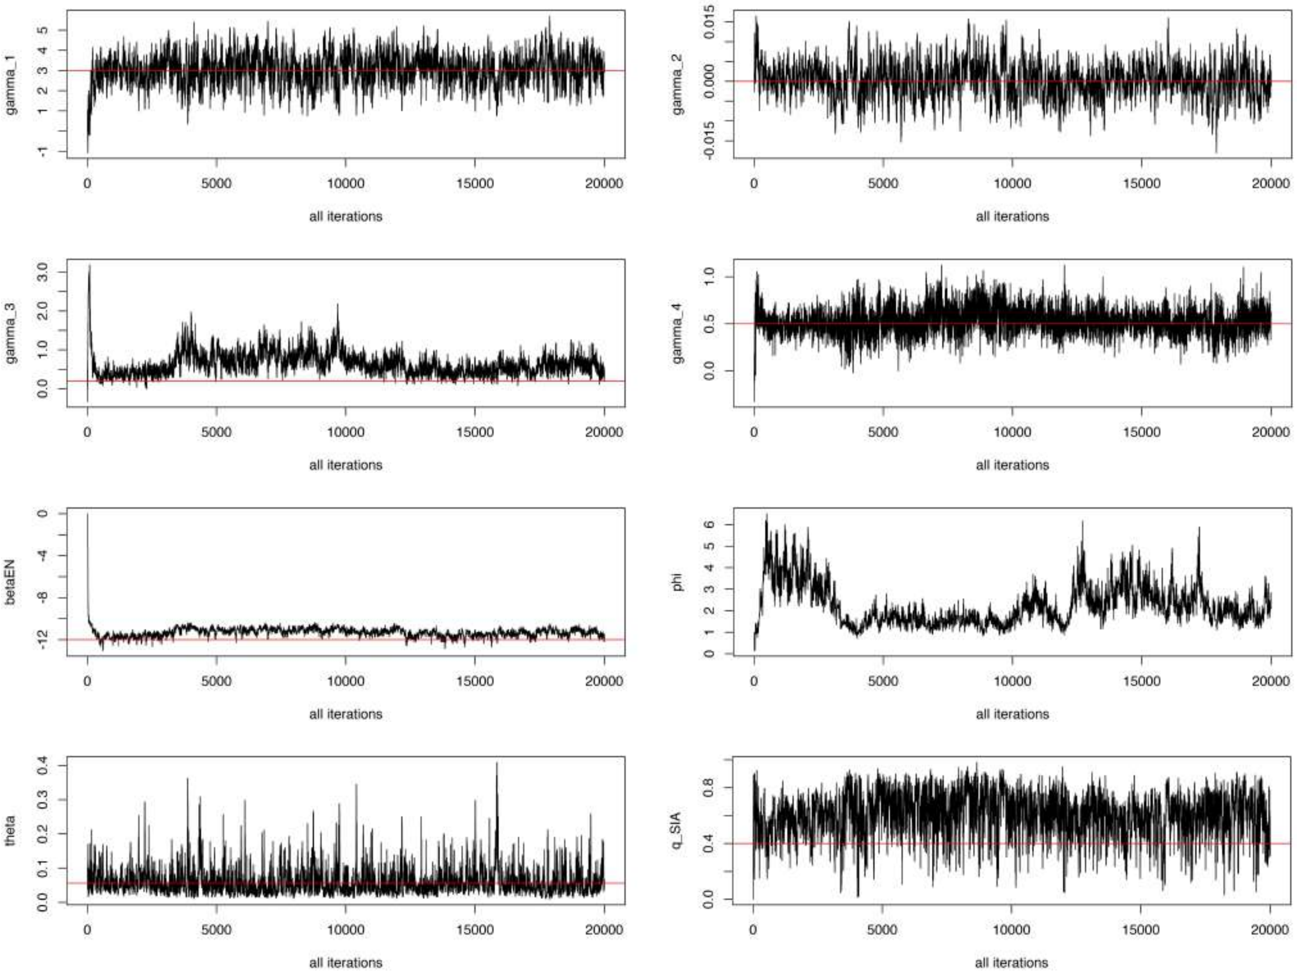


Web Figure 8: Traceplots of posterior samples of model parameters in the simulation study computed with uncertainty propagation for when the reporting rate $\rho = 0.7$.

## Web Figure 9

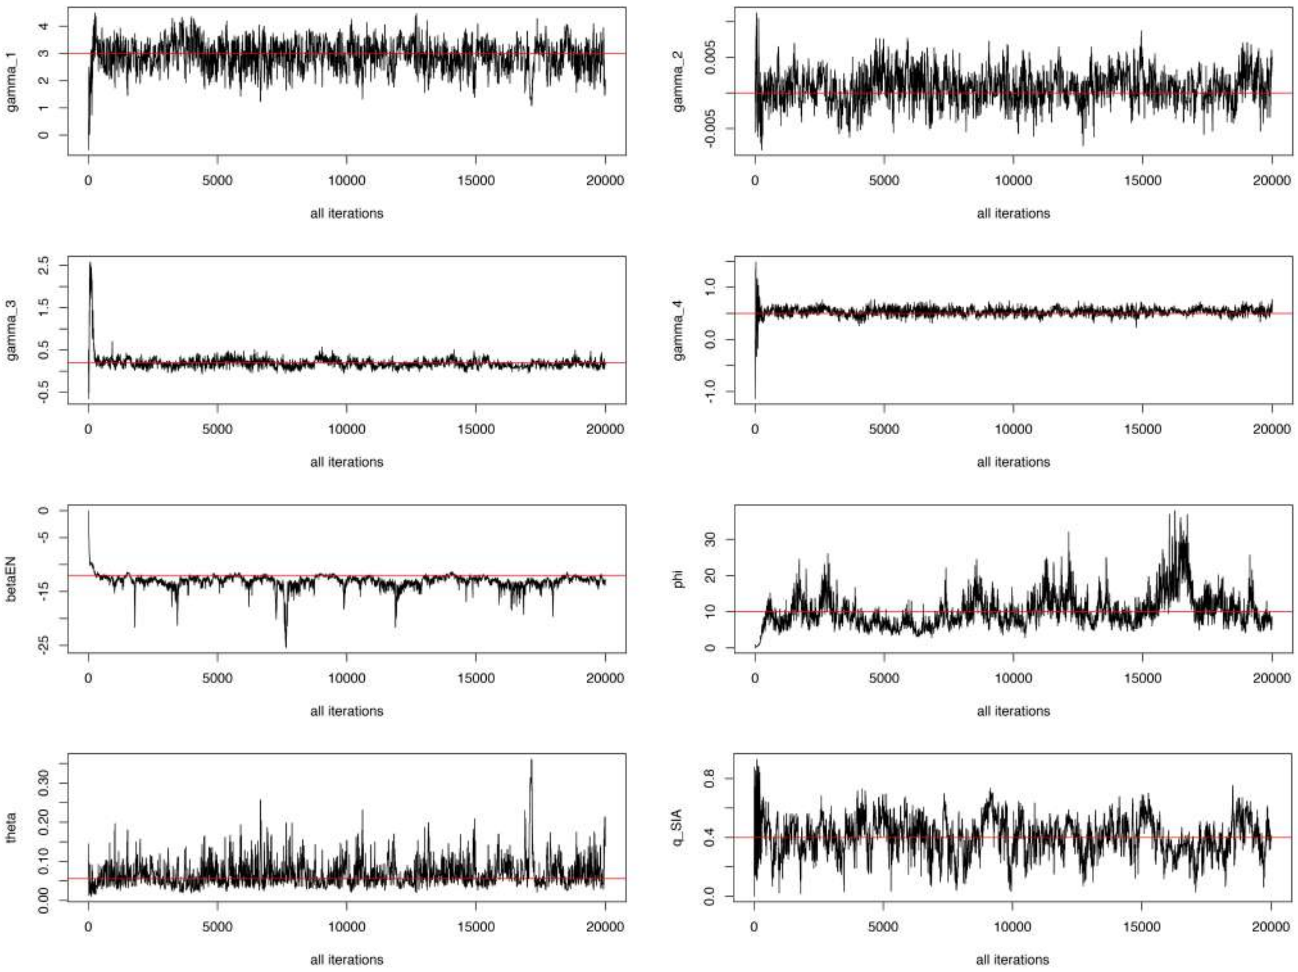


Web Figure 9: Traceplots of posterior samples of model parameters in the simulation study computed without uncertainty propagation (i.e., true $\rho$ plugged-in) where reporting rate $\rho = 0.01$.

## Web Figure 10

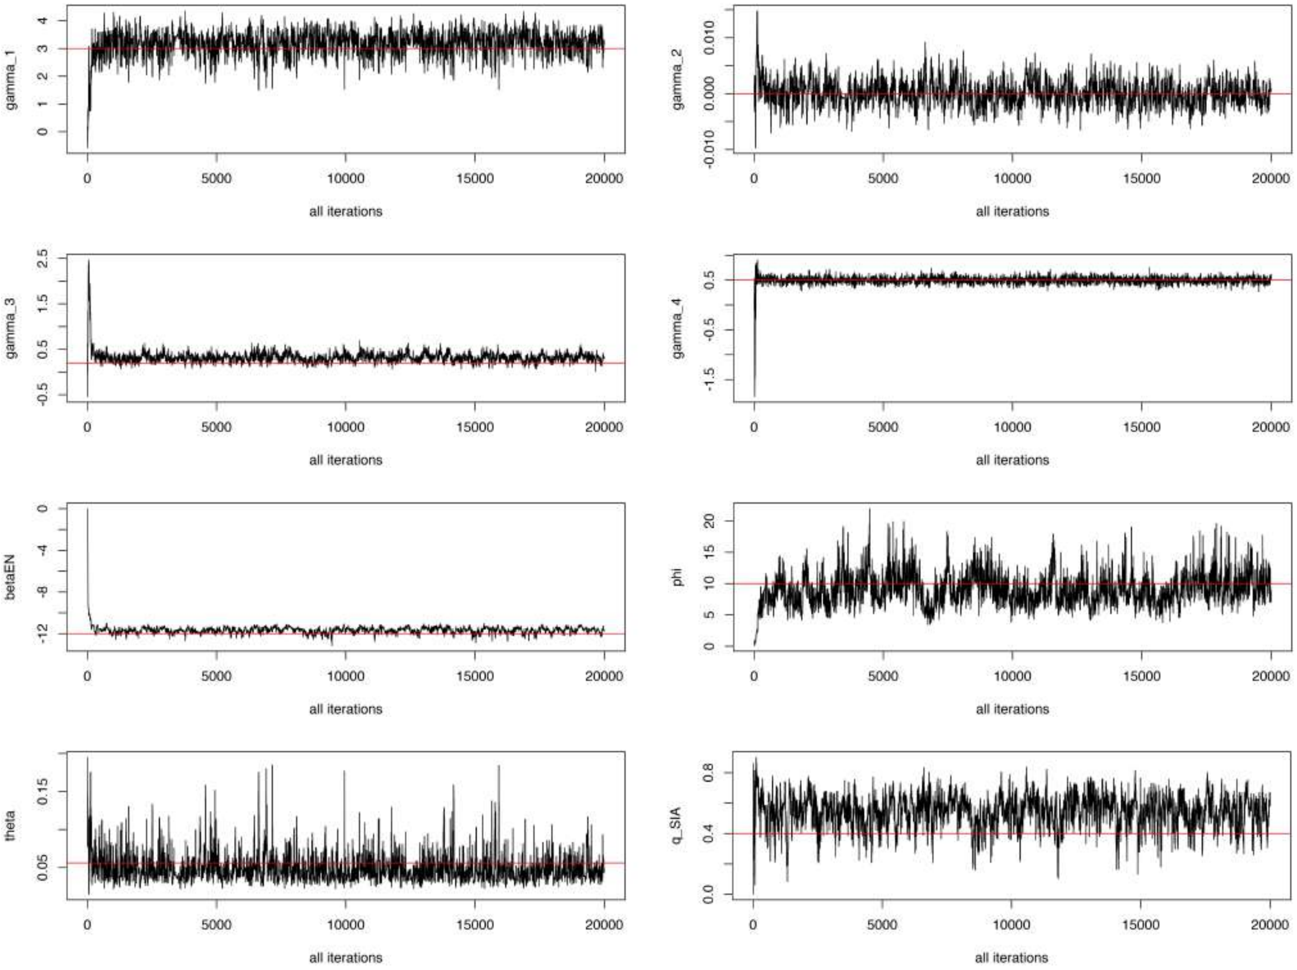


Web Figure 10: Traceplots of posterior samples of model parameters in the simulation study computed without uncertainty propagation (i.e., true $\rho$ plugged-in) where reporting rate $\rho = 0.1$.

# Web Figure 11

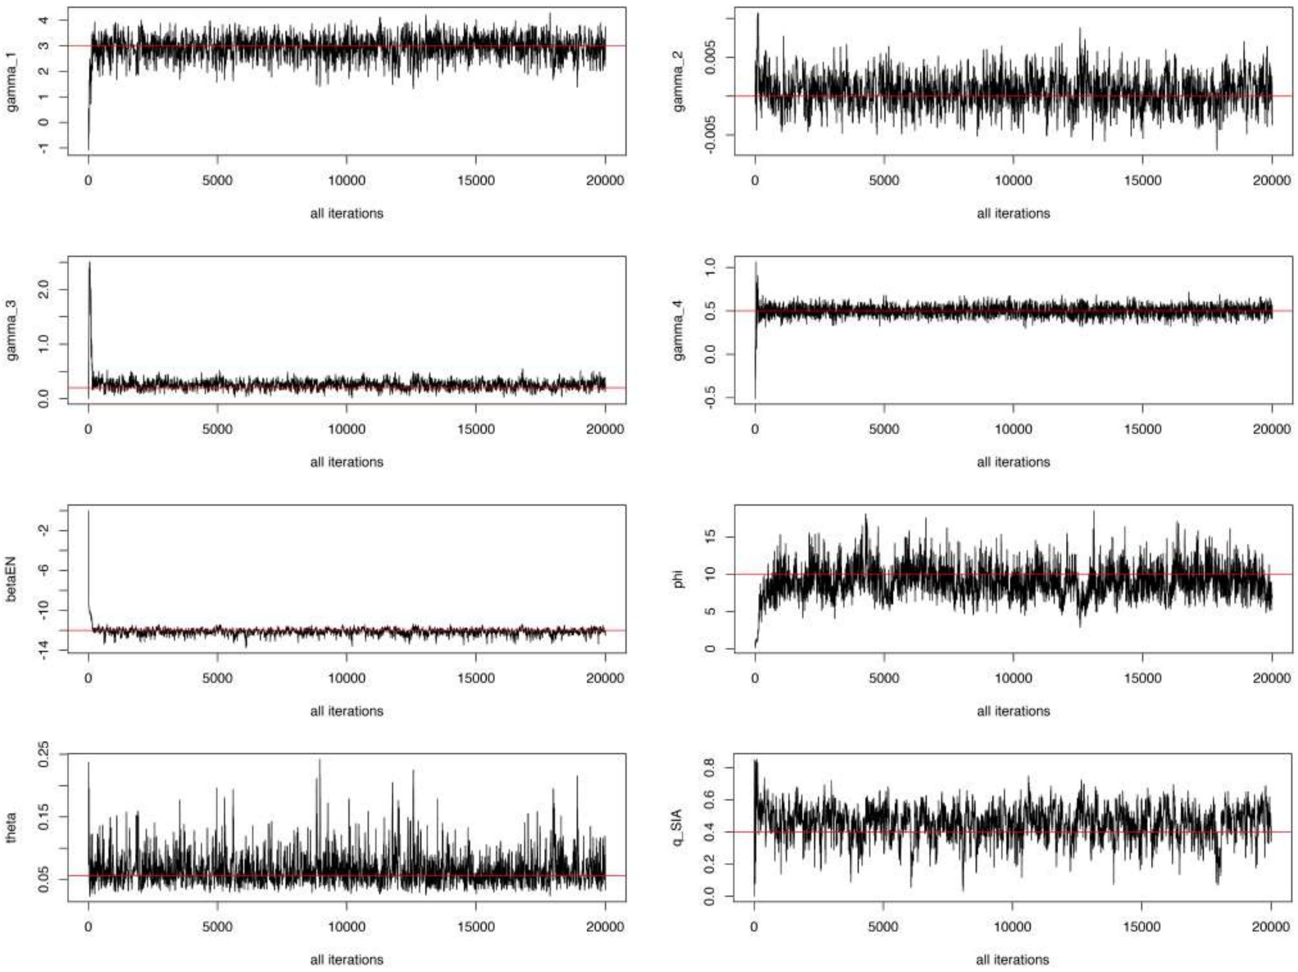


Web Figure 11: Traceplots of posterior samples of model parameters in the simulation study computed without uncertainty propagation (i.e., true $\rho$ plugged-in) where reporting rate $\rho = 0.3$.

# Web Figure 12

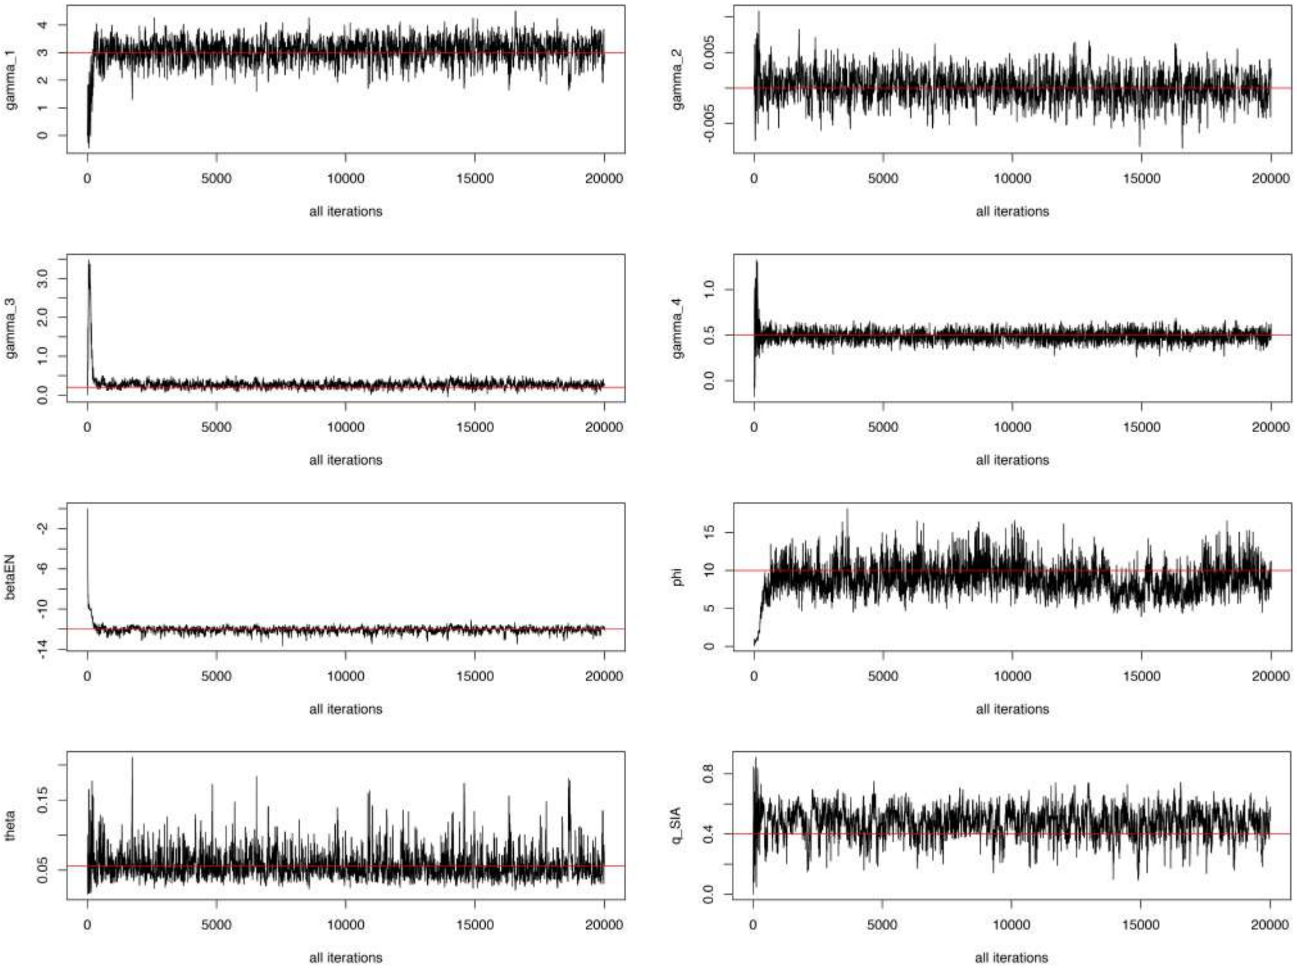


Web Figure 12: Traceplots of posterior samples of model parameters in the simulation study computed without uncertainty propagation (i.e., true $\rho$ plugged-in) where reporting rate $\rho = 0.5$.

## Web Figure 13

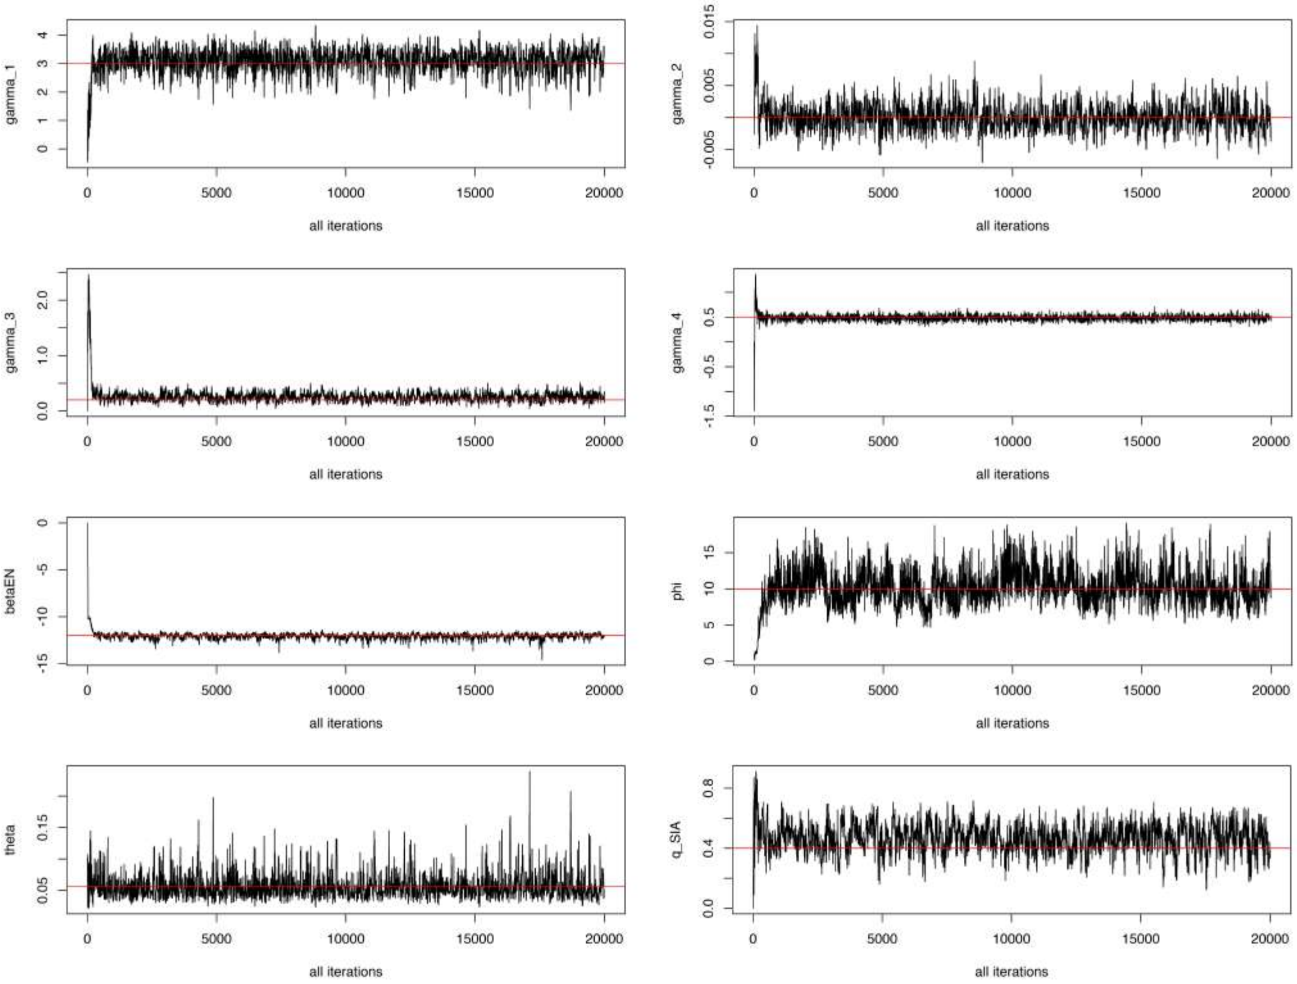


Web Figure 13: Traceplots of posterior samples of model parameters in the simulation study computed without uncertainty propagation (i.e., true $\rho$ plugged-in) where reporting rate $\rho = 0.7$.

# Web Figure 14

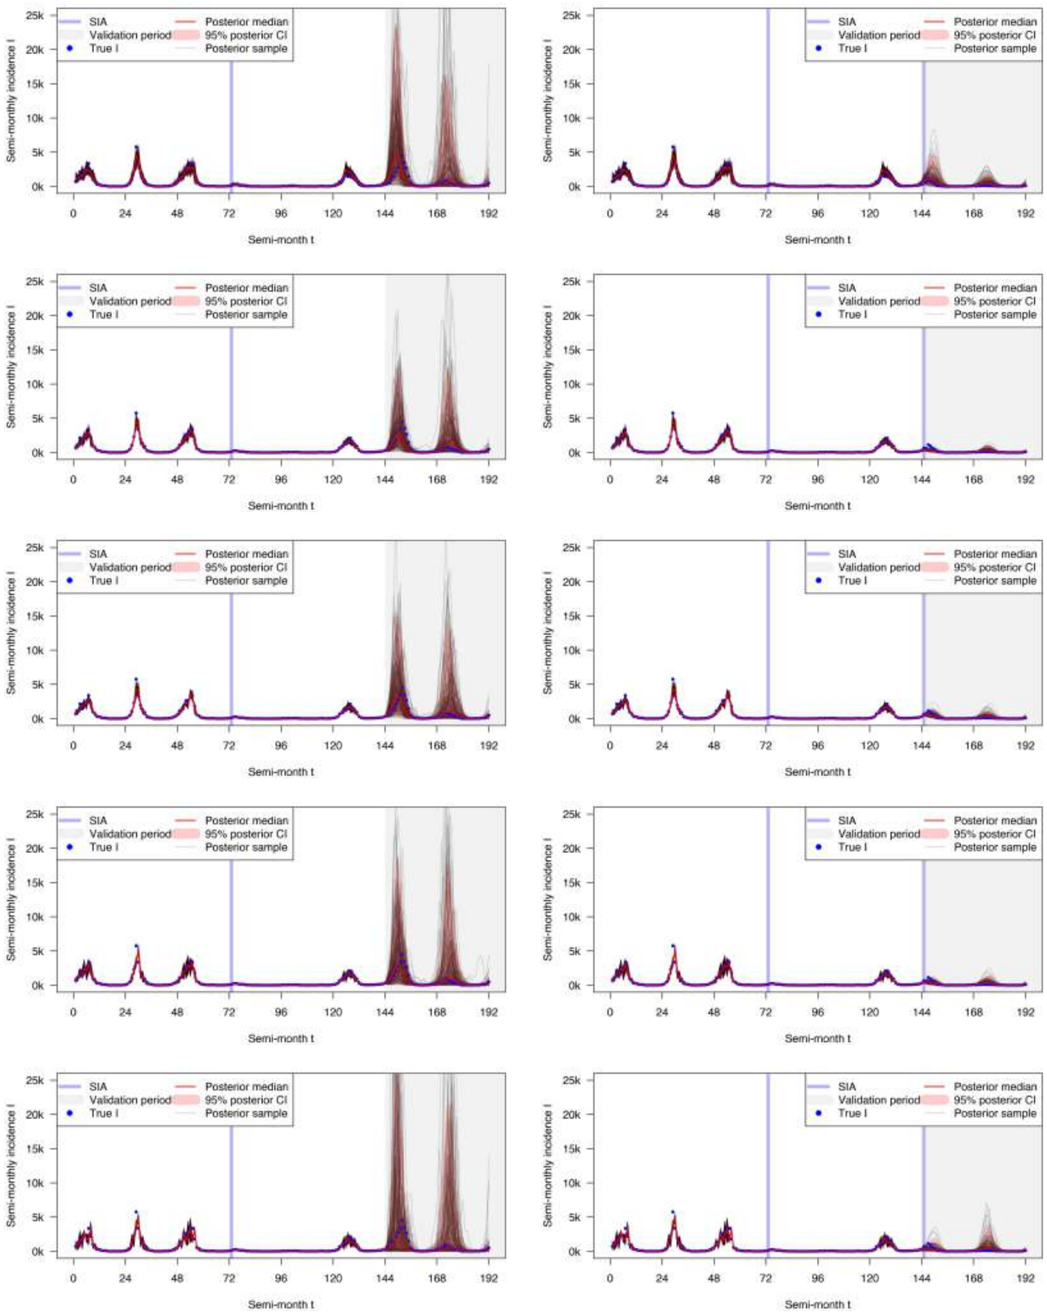


Web Figure 14: The simulated true values, posterior medians, 95% posterior CIs/predictive intervals and 200 randomly selected posterior samples of the underlying measles incidence computed with uncertainty propagation for when the reporting rate is 0.01, 0.1, 0.3, 0.5 and 0.7 (from top to bottom), without (left) and with (right) a “planned” SIA at the beginning of the forecast period, respectively.

## Web Figure 15

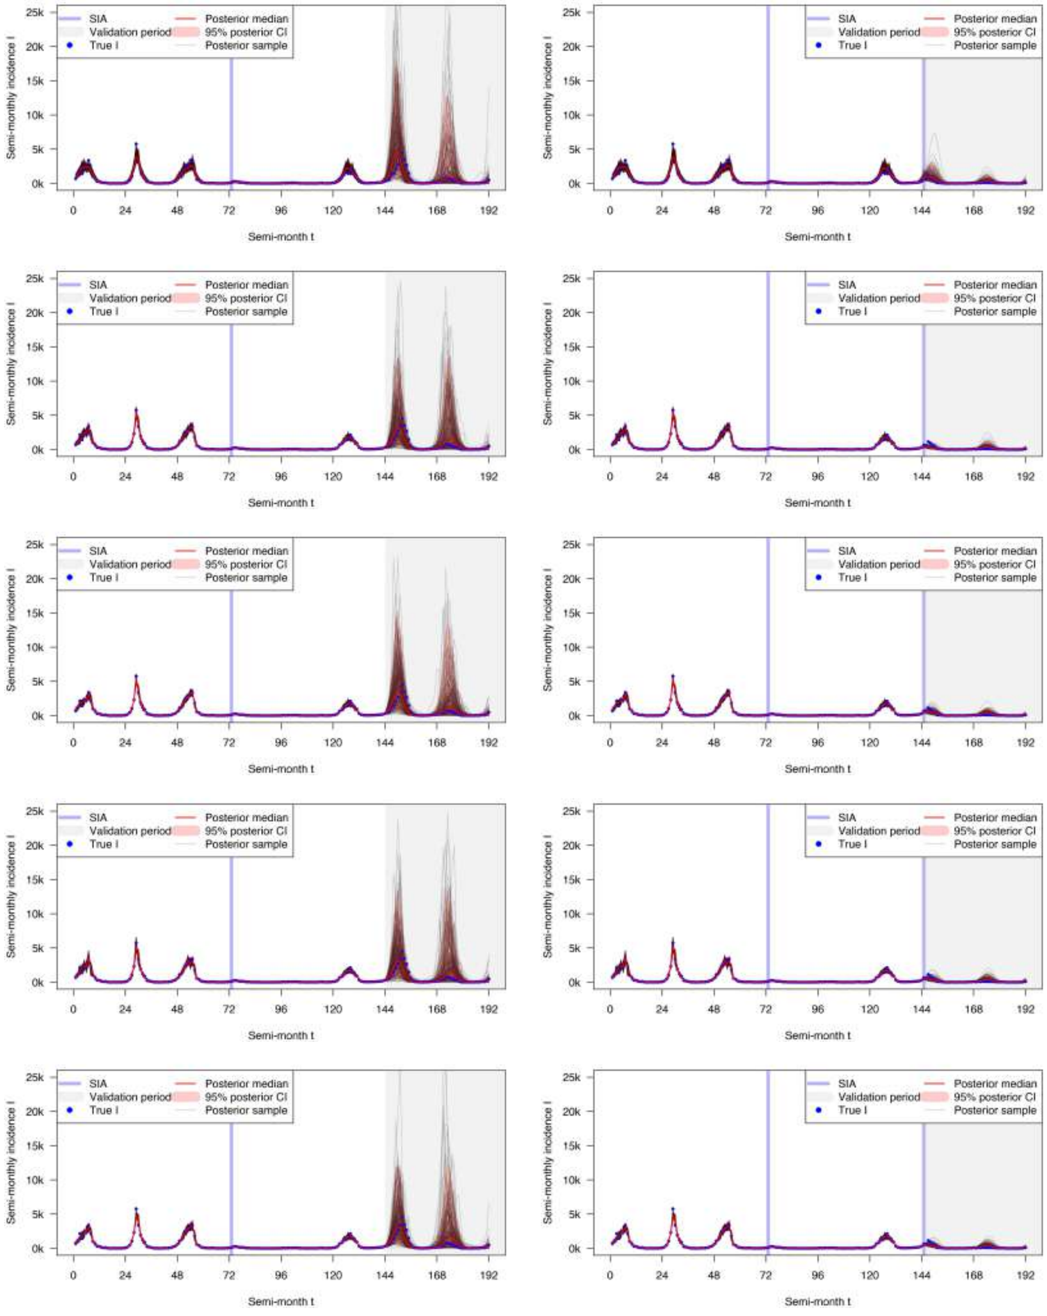


Web Figure 15: The simulated true values, posterior medians, 95% posterior CIs/predictive intervals and 200 randomly selected posterior samples of the underlying measles incidence computed without uncertainty propagation (i.e., true $\rho$ plugged in) for when the reporting rate is 0.01, 0.1, 0.3, 0.5 and 0.7 (from top to bottom), without (left) and with (right) a “planned” SIA at the beginning of the forecast period, respectively.

# Web Figure 16

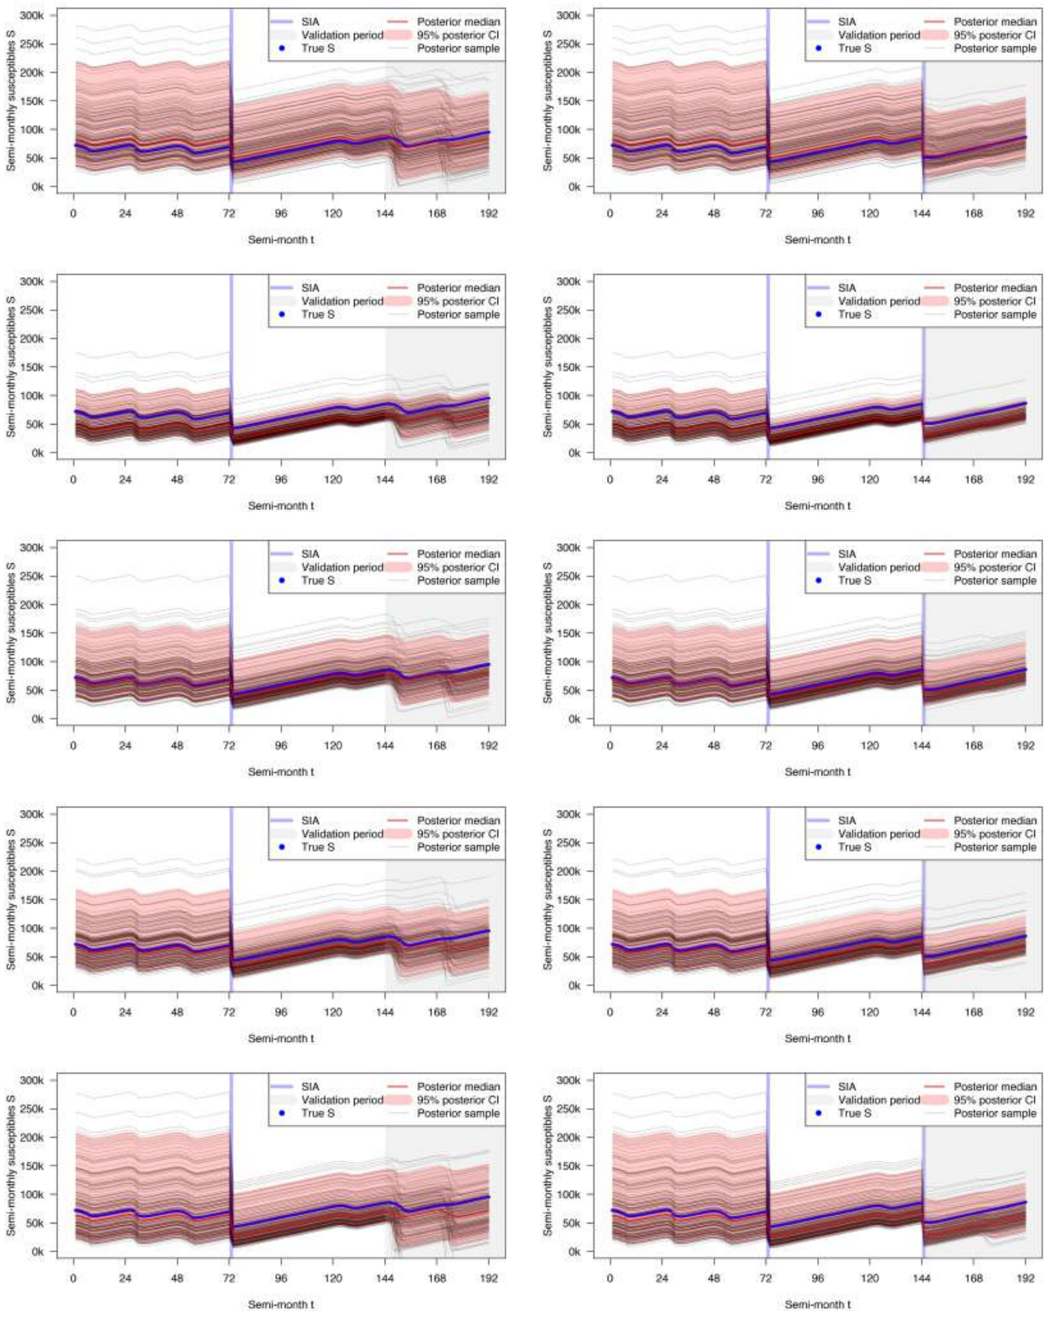


Web Figure 16: The simulated true values, posterior medians, 95% posterior CIs/predictive intervals and 200 randomly selected posterior samples of the underlying susceptible population computed with uncertainty propagation for when the reporting rate is 0.01, 0.1, 0.3, 0.5 and 0.7 (from top to bottom), without (left) and with (right) a "planned" SIA at the beginning of the forecast period, respectively.

# Web Figure 17

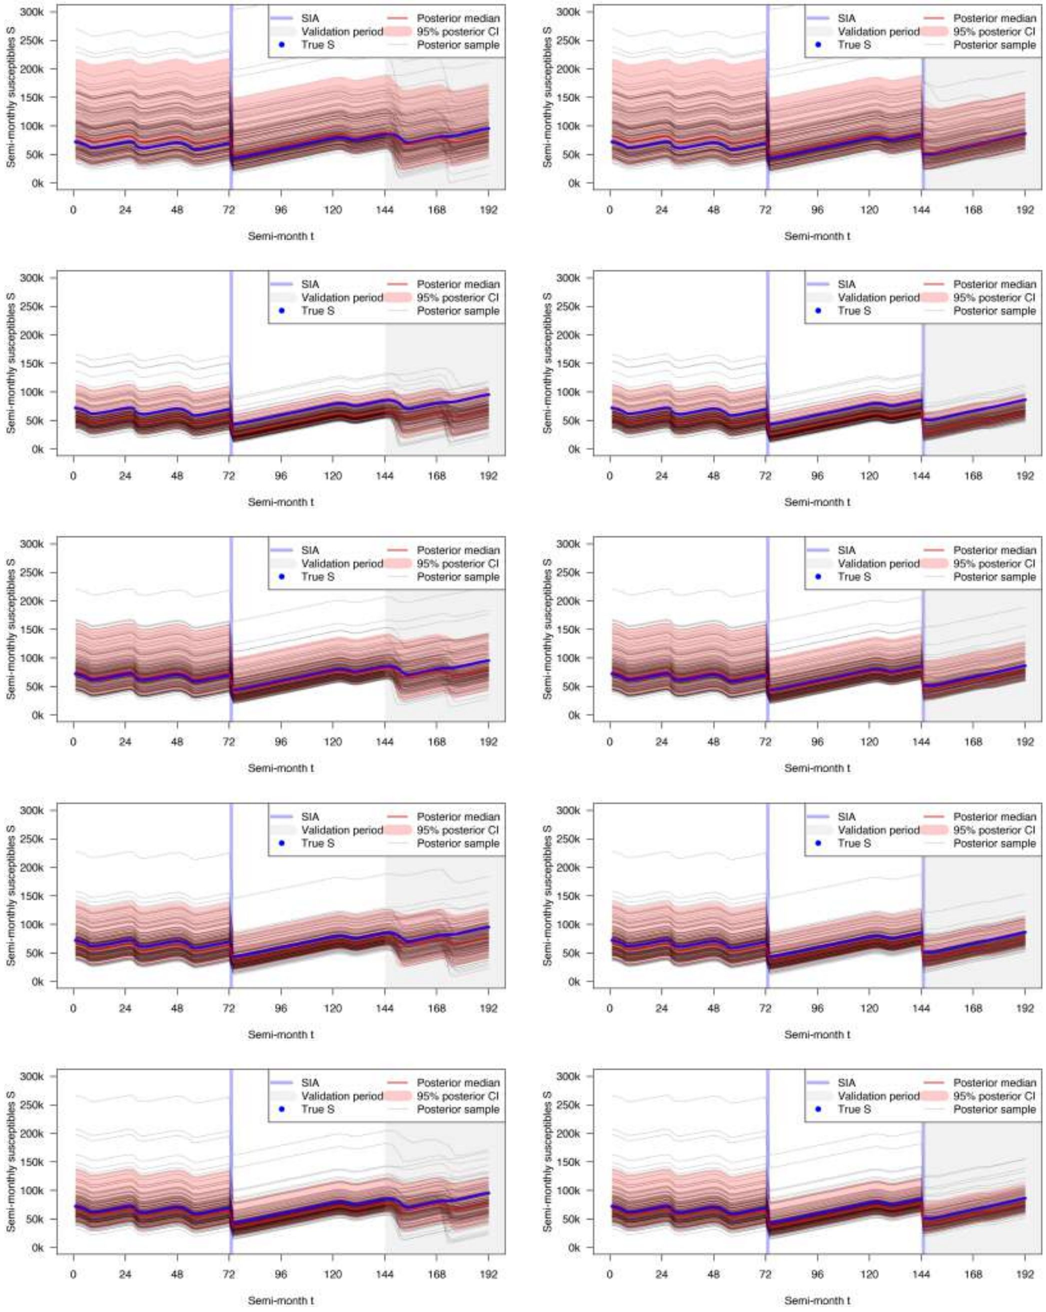


Web Figure 17: The simulated true values, posterior medians, 95% posterior CIs/predictive intervals and 200 randomly selected posterior samples of the underlying susceptible population computed without uncertainty propagation (i.e., true $\rho$ plugged in) for when the reporting rate is 0.01, 0.1, 0.3, 0.5 and 0.7 (from top to bottom), without (left) and with (right) a "planned" SIA at the beginning of the forecast period, respectively.

## Web Figure 18

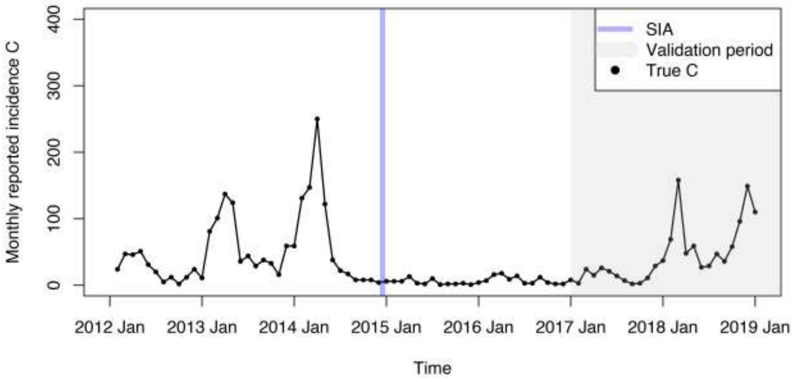


Web Figure 18: The monthly reported measles incidence in Benin between January 2012 and December 2018.

## Web Figure 19

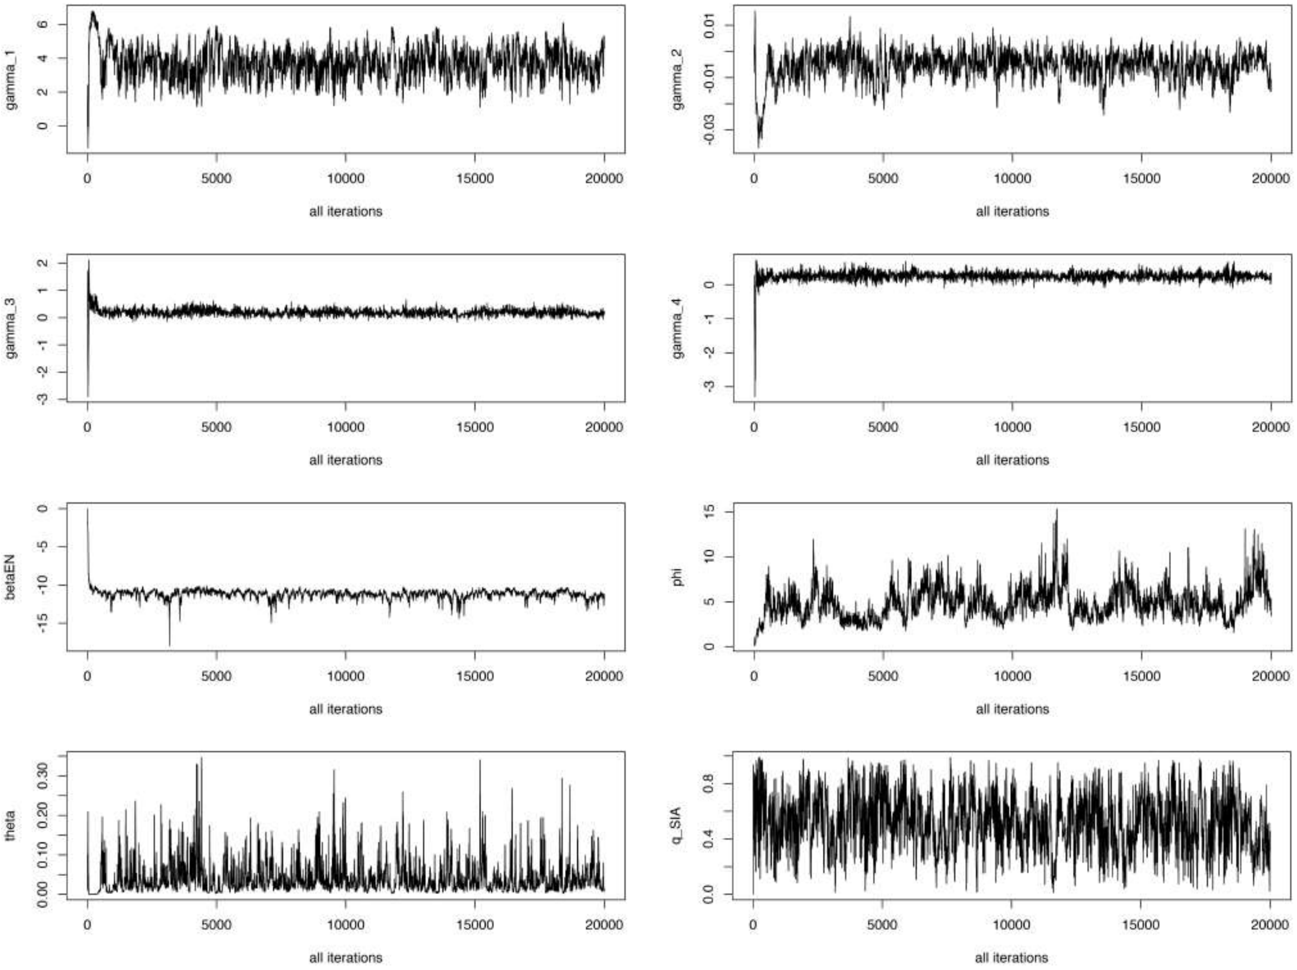


Web Figure 19: Traceplots of posterior samples of model parameters in the Benin analysis.

# References


Anderson, R. M., Anderson, B., and May, R. M. (1992). *Infectious Diseases of Humans: Dynamics and Control.* Oxford University Press.

Begon, M., Bennett, M., Bowers, R. G., French, N. P., Hazel, S., and Turner, J. (2002). A clarification of transmission terms in host-microparasite models: numbers, densities and areas. *Epidemiology & Infection* **129,** 147–153.

Bjørnstad, O. N., Finkenstädt, B. F., and Grenfell, B. T. (2002). Dynamics of measles epidemics: estimating scaling of transmission rates using a time series SIR model. *Ecological Monographs* **72,** 169–184.

Cox, D. R. and Miller, H. D. (1977). *The Theory of Stochastic Processes*, volume 134. CRC Press.

Feller, W. (1950). *An Introduction to Probability Theory and Its Applications.* New York: John Wiley & Sons Inc.

Ferrari, M. J., Grais, R. F., Bharti, N., Conlan, A. J., Bjørnstad, O. N., Wolfson, L. J., Guerin, P. J., Djibo, A., and Grenfell, B. T. (2008). The dynamics of measles in sub-Saharan Africa. *Nature* **451,** 679.

Finkenstädt, B. F. and Grenfell, B. T. (2000). Time series modelling of childhood diseases: a dynamical systems approach. *Journal of the Royal Statistical Society: Series C (Applied Statistics)* **49,** 187–205.

Glass, K., Xia, Y., and Grenfell, B. (2003). Interpreting time-series analyses for continuous-time biological modelsâĂŤmeasles as a case study. *Journal of Theoretical Biology* **223,** 19–25.

Grenfell, B. T., Bjørnstad, O. N., and Finkenstädt, B. F. (2002). Dynamics of measles epidemics: scaling noise, determinism, and predictability with the TSIR model. *Ecological Monographs* **72,** 185–202.

Mahmud, A. S., Metcalf, C. J. E., and Grenfell, B. T. (2017). Comparative dynamics, seasonality in transmission, and predictability of childhood infections in Mexico. *Epidemiology & Infection* **145,** 607–625.

Metcalf, C., Bjørnstad, O., Ferrari, M., Klepac, P., Bharti, N., Lopez-Gatell, H., and Grenfell, B. (2011). The epidemiology of rubella in Mexico: seasonality, stochasticity and regional variation. *Epidemiology & Infection* **139,** 1029–1038.

Metcalf, C., Cohen, C., Lessler, J., McAnerney, J., Ntshoe, G., Puren, A., Klepac, P., Tatem, A., Grenfell, B., and Bjørnstad, O. (2013). Implications of spatially heterogeneous vaccination coverage for the risk of congenital rubella syndrome in South Africa. *Journal of the Royal Society Interface* **10,** 20120756.

Morton, A. and Finkenstädt, B. F. (2005). Discrete time modelling of disease incidence time series by using Markov chain Monte Carlo methods. *Journal of the Royal Statistical Society: Series C (Applied Statistics)* **54,** 575–594.

Wakefield, J., Dong, T. Q., and Minin, V. N. (2019). Spatio-temporal analysis of surveillance data. In Held, L., Hens, N., O'Neill, P. D., and Wallinga, J., editors, *Handbook of Infectious Disease Data Analysis*, pages 455–476. CRC Press.
